# Supplementary material for: Constraining nuclear matter parameters with GW170817
Source: arXiv:1812.08910 ancillary file (2021-01-18)
Supplement: Supplementary file 1 [file Erratum.pdf]

# Erratum: Constraining nuclear matter parameters with GW170817 [Phys.Rev. D99 (2019)]

Zack Carson,<sup>1</sup> Andrew W. Steiner,<sup>2,3</sup> and Kent Yagi<sup>1</sup>

<sup>1</sup>*Department of Physics, University of Virginia, Charlottesville, Virginia 22904, USA*

<sup>2</sup>*Department of Physics and Astronomy, University of Tennessee, Knoxville, TN 37996, USA*

<sup>3</sup>*Physics Division, Oak Ridge National Laboratory, Oak Ridge, TN 37831, USA*

(Dated: March 23, 2020)

In this erratum, we correct the method used previously to calculate posterior probability distributions on nuclear matter parameters. In particular, previously they were computed by marginalizing over two-dimensional probability distributions between nuclear parameters and the tidal deformability. We correct this by instead considering the one-dimensional conditional probability distribution between the former given an observation of the latter.

## I. CONSTRAINT ESTIMATION VIA LIGO POSTERIOR DISTRIBUTIONS

In [1], we computed posterior probability distributions on nuclear matter parameters  $Y$  by marginalizing over the two dimensional probability distributions  $P(Y, \tilde{\Lambda})$  with the mass-weighted tidal deformability  $\tilde{\Lambda}$  multiplied by the posterior probability distribution on  $\tilde{\Lambda}$  from the LIGO/Virgo collaboration's (LVC's) gravitational wave (GW) observation of GW170817 [2]. In particular, we find that this method needs to be corrected from a dimensional analysis point of view, and we instead consider the conditional one-dimensional probability distribution on nuclear matter parameters given tidal deformability observation  $\tilde{\Lambda}_{\text{obs}}$ .

With the new method, we once again begin by generating the 2-dimensional probability distribution between  $\tilde{\Lambda}$  and the nuclear parameters, taking into account the specific covariances between them. For the example of  $K_{\text{sym},0}$  the distribution is given by

$$P(\tilde{\Lambda}, K_{\text{sym},0}) = \frac{1}{2\pi\sqrt{|\Sigma|}} e^{-\frac{1}{2}(x-\mu)^T \Sigma^{-1}(x-\mu)}, \quad (1)$$

where  $x$  is the 2-dimensional vector containing  $\tilde{\Lambda}$  and the given nuclear parameter,  $\mu$  is the 2-dimensional vector containing the expected values of  $x$ , and  $\Sigma$  is the  $2 \times 2$  covariance matrix defined with elements given by Eq. (10) of [1]. This distribution is displayed in e.g. Fig. 8 of [1] for each nuclear parameter, where the high degree of covariance between the variables is visible.

Following this, we compute the conditional probability distributions on nuclear matter parameters  $Y$  given a tidal observation of  $\tilde{\Lambda}_{\text{obs}}$ . Following e.g. Ref. [3], the one-dimensional conditional probability distribution on nuclear parameter  $Y$  is then given by

$$P(Y|\tilde{\Lambda}_{\text{obs}}) \sim \mathcal{N}\left(\mu_Y + \frac{\sigma_Y}{\sigma_{\tilde{\Lambda}_{\text{obs}}}} C(\tilde{\Lambda}_{\text{obs}} - \mu_{\tilde{\Lambda}_{\text{obs}}}), (1 - C^2)\sigma_Y^2\right). \quad (2)$$

In the above expression,  $\mathcal{N}(\mu, \sigma^2)$  is the normal distribution with mean and variance  $\mu$  and  $\sigma^2$ ,  $\mu_A$  and  $\sigma_A^2$  are the mean and variances of  $Y$  and  $\tilde{\Lambda}_{\text{obs}}$ , and  $C$  is the Pearson correlation coefficient given in Eq. (9) of [1].

Finally, we extract the one-dimensional probability distributions on  $K_0 + \alpha L_0$ ,  $M_0 + \beta L_0$ , and  $K_{\text{sym},0}$  by combining the one-dimensional conditional distributions  $P(Y|\tilde{\Lambda})$  found in Eq. (2) with the probability distribution  $P_{\text{LIGO}}(\tilde{\Lambda})$  on  $\tilde{\Lambda}$  derived by the LIGO Collaboration in Ref. [4] for GW170817. For example, the posterior probability distribution on  $K_0 + \alpha L_0$  is given by:

$$P(K_0 + \alpha L_0) = \int_{-\infty}^{\infty} P(K_0 + \alpha L_0|\tilde{\Lambda}) P_{\text{LIGO}}(\tilde{\Lambda}) d\tilde{\Lambda}, \quad (3)$$

and similarly for  $M_0 + \beta L_0$  and  $K_{\text{sym},0}$ . Additionally, as was done [1], we find the probability distributions on  $K_0$  and  $M_0$  by performing one last integration over the prior probability distribution of  $L_0$ , assumed to be Gaussian with standard deviation  $\sigma = \frac{1}{2}(80 + 36)$  and mean  $\mu = \frac{1}{2}(80 - 36)$  [5]. For example, the probability distribution on  $K_0$  is given by:

$$P(K_0) = \int_{-\infty}^{\infty} P(K_0 + \alpha L_0) P(L_0) dL_0, \quad (4)$$

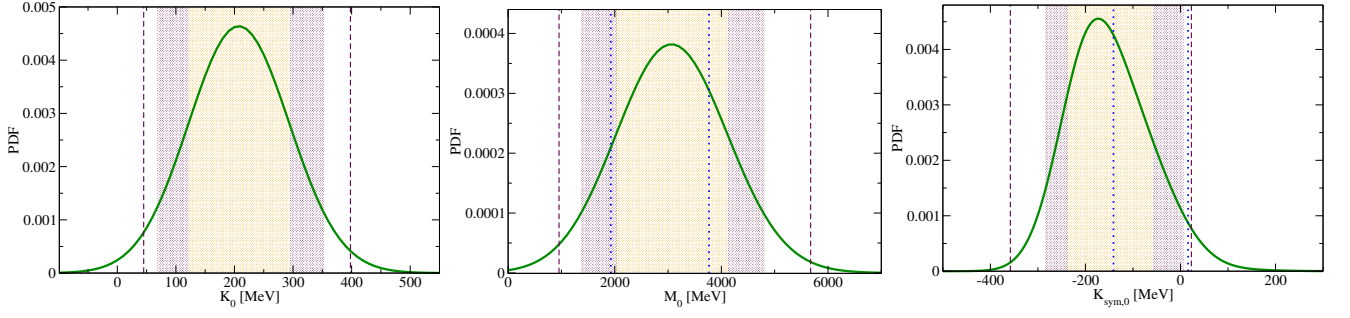

FIG. 1. Updated Fig. 10 from [1]. Posterior distributions on the nuclear incompressibility  $K_0$  and its slope  $M_0$ , and the curvature of symmetry energy  $K_{\text{sym},0}$  derived by integrating over the product of one-dimensional conditional probability distributions ( $P(K_0 + \alpha L_0 | \tilde{\Lambda})$ ,  $P(M_0 + \beta L_0 | \tilde{\Lambda})$ , and  $P(K_{\text{sym},0} | \tilde{\Lambda})$ ) and  $P_{\text{LIGO}}(\tilde{\Lambda})$  from [4]. Further, for the linear combinations of  $K_0 + \alpha L_0$  and  $M_0 + \beta L_0$ , one more integration over the probability distribution of  $30 \text{ MeV} \leq L_0 \leq 86 \text{ MeV}$  was required to directly find the posterior distributions on  $K_0$  and  $M_0$ . Overlayed are the resulting 68% and 90% confidence intervals in orange and maroon respectively, as well as the corresponding bounds calculated in [1] with the less accurate method of computing constraints. Additionally shown in dotted blue are the corresponding bounds on  $M_0$  and  $K_{\text{sym},0}$  computed by Ref. [6], using priors of  $\tilde{\Lambda} \in [70, 720]$  and  $L_0 \in [30, 86] \text{ MeV}$ .

with  $\alpha = 2.27$ .

The new results of these computations are shown in Fig. 1 for the more conservative priors on  $L_0$ . We observe that the  $K_0$ ,  $M_0$ , and  $K_{\text{sym},0}$  parameters now obey distributions that look like skewed Gaussians centered at  $K_0 = 208^{+86}_{-85} \text{ MeV}$ ,  $M_0 = 3075^{+1045}_{-1033} \text{ MeV}$ , and  $K_{\text{sym},0} = -156^{+97}_{-81} \text{ MeV}$  (68% standard deviations). This results in 90% confidence intervals of  $69 \text{ MeV} \leq K_0 \leq 352 \text{ MeV}$ ,  $1371 \text{ MeV} \leq M_0 \leq 4808 \text{ MeV}$ , and  $-285 \text{ MeV} \leq K_{\text{sym},0} \leq 7 \text{ MeV}$ . In comparison to [1] where we found nearly-Gaussian probability distributions, we find such constraints to be skewed more to smaller values of nuclear parameters, especially for the higher-order parameter  $K_{\text{sym},0}$ . However, we find that the range of probable values remain mostly unchanged from the original analysis.

TABLE I. Updated Tab. I from [1]. GW170817 constraints on the incompressibility  $K_0$  (top row), its slope  $M_0$  (middle row), and the symmetry energy curvature  $K_{\text{sym},0}$  for 4 different sets of priors on  $L_0$  [5, 7–9], and  $\tilde{\Lambda}$  [2, 10]. These quantities are computed using two different methods: (i) a simple linear regression estimation described in [1] (labeled “Method 1” on the right column), and (ii) a comprehensive computation of the nuclear parameter posterior probability distributions described here (labeled “Method 2” on the left column).

| $L_0 \text{ [MeV]} \backslash \tilde{\Lambda}$ | Method 2                                                    | Method 1                                                     |                                                              |
|------------------------------------------------|-------------------------------------------------------------|--------------------------------------------------------------|--------------------------------------------------------------|
|                                                | $\tilde{\Lambda}$ Posterior Distribution [4]                | 70–720 [2]                                                   | 279–822 [10]                                                 |
| 40–62 [7–9]                                    | $69 \text{ MeV} \leq K_0 \leq 352 \text{ MeV}$              | $100 \text{ MeV} \leq K_0 \leq 375 \text{ MeV}$              | $118 \text{ MeV} \leq K_0 \leq 388 \text{ MeV}$              |
|                                                | $1371 \text{ MeV} \leq M_0 \leq 4808 \text{ MeV}$           | $1538 \text{ MeV} \leq M_0 \leq 5433 \text{ MeV}$            | $1849 \text{ MeV} \leq M_0 \leq 5609 \text{ MeV}$            |
|                                                | $-285 \text{ MeV} \leq K_{\text{sym},0} \leq 7 \text{ MeV}$ | $-358 \text{ MeV} \leq K_{\text{sym},0} \leq 23 \text{ MeV}$ | $-298 \text{ MeV} \leq K_{\text{sym},0} \leq 54 \text{ MeV}$ |
| 30–86 [5]                                      | $123 \text{ MeV} \leq K_0 \leq 330 \text{ MeV}$             | $45 \text{ MeV} \leq K_0 \leq 398 \text{ MeV}$               | $63 \text{ MeV} \leq K_0 \leq 411 \text{ MeV}$               |
|                                                | $1884 \text{ MeV} \leq M_0 \leq 4635 \text{ MeV}$           | $955 \text{ MeV} \leq M_0 \leq 5675 \text{ MeV}$             | $1266 \text{ MeV} \leq M_0 \leq 5852 \text{ MeV}$            |
|                                                | $-285 \text{ MeV} \leq K_{\text{sym},0} \leq 7 \text{ MeV}$ | $-358 \text{ MeV} \leq K_{\text{sym},0} \leq 23 \text{ MeV}$ | $-298 \text{ MeV} \leq K_{\text{sym},0} \leq 54 \text{ MeV}$ |

- 
- [1] Z. Carson, A. W. Steiner, and K. Yagi, *Phys. Rev.* **D99**, 043010 (2019), [arXiv:1812.08910 \[gr-qc\]](#).
  - [2] B. P. Abbott *et al.* (LIGO Scientific, Virgo), *Phys. Rev.* **X9**, 011001 (2019), [arXiv:1805.11579 \[gr-qc\]](#).
  - [3] J. L. Jensen, *Statistics for petroleum engineers and geoscientists* (Elsevier, 2007).
  - [4] B. P. Abbott *et al.* (LIGO Scientific, Virgo), *Phys. Rev.* **X9**, 011001 (2019), [arXiv:1805.11579 \[gr-qc\]](#).
  - [5] M. Oertel, M. Hempel, T. Klähn, and S. Typel, *Rev. Mod. Phys.* **89**, 015007 (2017).
  - [6] T. Malik, N. Alam, M. Fortin, C. Providencia, B. K. Agrawal, T. K. Jha, B. Kumar, and S. K. Patra, *Phys. Rev.* **C98**, 035804 (2018), [arXiv:1805.11963 \[nucl-th\]](#).
  - [7] J. M. Lattimer and Y. Lim, *The Astrophysical Journal* **771**, 51 (2013).
  - [8] J. M. Lattimer and A. W. Steiner, *The European Physical Journal A* **50** (2014), [10.1140/epja/i2014-14040-y](#).
  - [9] I. Tews, J. M. Lattimer, A. Ohnishi, and E. E. Kolomeitsev, *The Astrophysical Journal* **848**, 105 (2017).
  - [10] M. W. Coughlin, T. Dietrich, B. Margalit, and B. D. Metzger, *Mon. Not. Roy. Astron. Soc.* **489**, L91 (2019), [arXiv:1812.04803 \[astro-ph.HE\]](#).
